# Supplementary material for: Cross-Scan Mamba with Masked Training for Robust Spectral Imaging
Source: arXiv:2408.00629 source file (2024-12-06)
Supplement: Supplementary file 1 [file X_suppl.tex]

\clearpage
\setcounter{page}{1}
\maketitlesupplementary

\section{Mask Degradation Estimation Module}
\subsection{Simulation Scenario}
In previous work, mask degradation estimation has demonstrated significant effectiveness in the simulation reconstruction experiment. Several studies have built upon \cite{dauhst} to achieve further improvements, yielding more accurate parameters and prior estimations. For instance, the mask residual estimation proposed by \cite{dernn} has significantly enhanced reconstruction outcomes in simulation scenarios, leaving no doubt about its effectiveness.

We also conducted some exploration on the mask estimation module. In the parameter estimation of DAUHST \cite{dauhst}, we change the estimated noise level from a constant to a tensor with the same size as the input to achieve a more precise estimation. Since the noise level in an image should actually be spatially variant, we can remove the Downsample and MaxPooling process and directly generate a pixel-level noise level map. Compared to the result of \cite{dauhst}, we indeed make some progress.

\begin{table}[H]
\vspace{-3mm}
\centering
    \caption{\footnotesize Comparisons of constant and map in noise level with the 3stg model PSNR, SSIM, FLOPs, and Params.}
\vspace{-2mm}
\label{tab:smallmodel}
 
\setlength{\tabcolsep}{2.4pt}
	\resizebox{0.37\textwidth}{!}
	{
	\begin{tabular}{l c c c}
				\toprule
				\rowcolor{color3}Framework &~Constant~  &~Noise Level Map~   \\
				\midrule
				PSNR &38.68   &\bf 38.96  \\
				SSIM  &0.972     &\bf0.976  \\
				Params (M)  &0.81     &\bf0.92   \\
				FLOPS (G) &29.25   &\bf30.80    \\
				\bottomrule
	\end{tabular}}
	\label{tab:ablations}
 \vspace{-3mm}
\end{table}

However, when the estimation module is modified to estimate the parameters of all stages iteratively instead of just in the initialization step, the increase in parameter count and computational complexity introduced by the noise level map method becomes prohibitively large. As a result, we ultimately decided to abandon this approach in the model.

\subsection{Real Scenario}
Previous works have overlooked the impact of Mask Degradation Estimation on the reconstruction of real-world scenes. In our paper, we compared three methods \cite{mst}, \cite{cst}, \cite{dauhst} and concluded that focusing on mask pattern recovery can overemphasize specific information, weakening resilience to other noise types and thus reducing the reconstruction ability of real scenes. However, this point cannot be rigorously established solely based on the comparison of these three methods. To address this, we further compare reconstruction results in DAUHST \cite{dauhst} with and without the degradation estimation module. Additionally, We also provide the reconstruction outcome of employing a more precise estimation method using in \cite{dernn}.

\begin{figure}[t]
  \centering
  
   \includegraphics[width=0.98\linewidth]{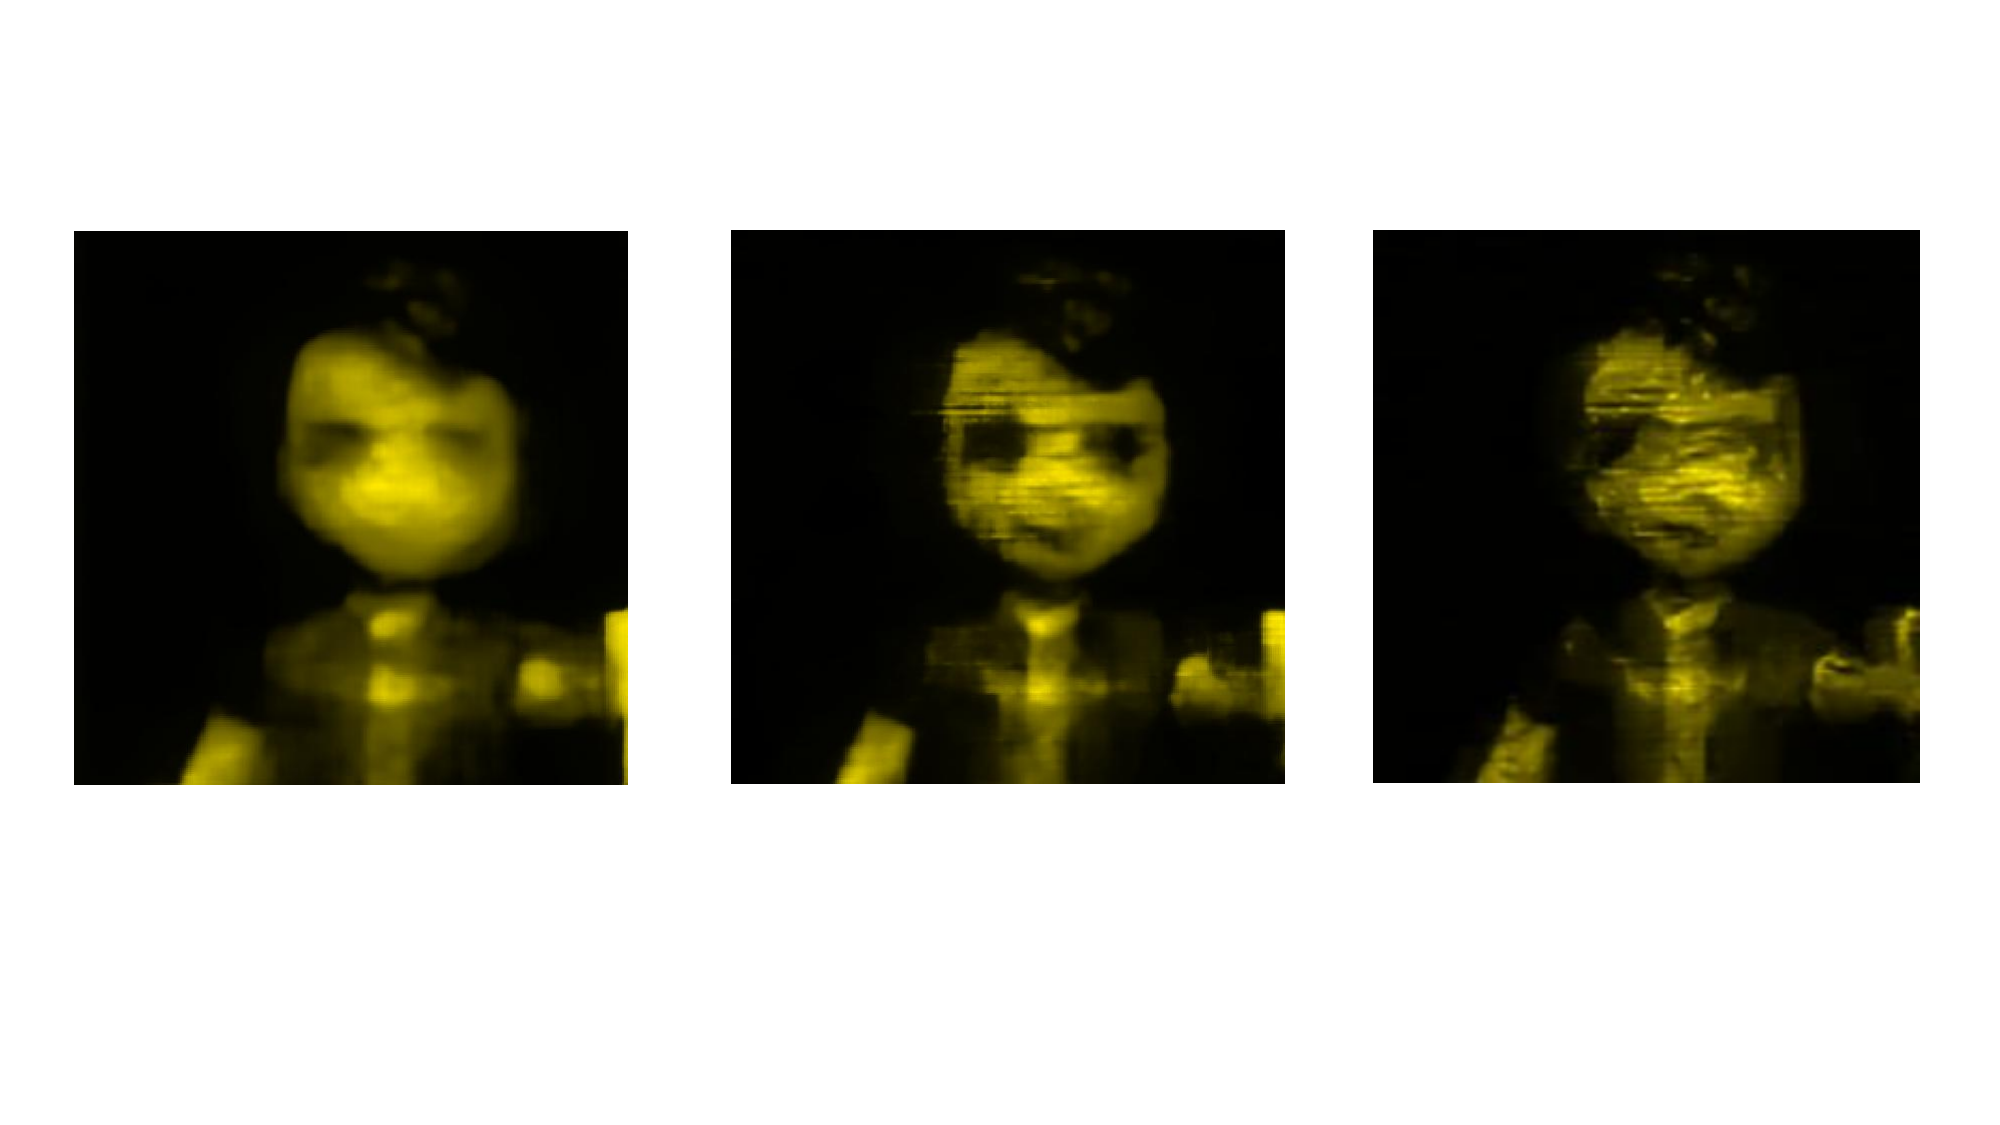}
   \label{fig:dauhst1}
   \vspace{-3.5mm}
\end{figure}

\begin{figure}[t]
  \centering
  \hspace{-2.5mm}
   \includegraphics[width=0.98\linewidth]{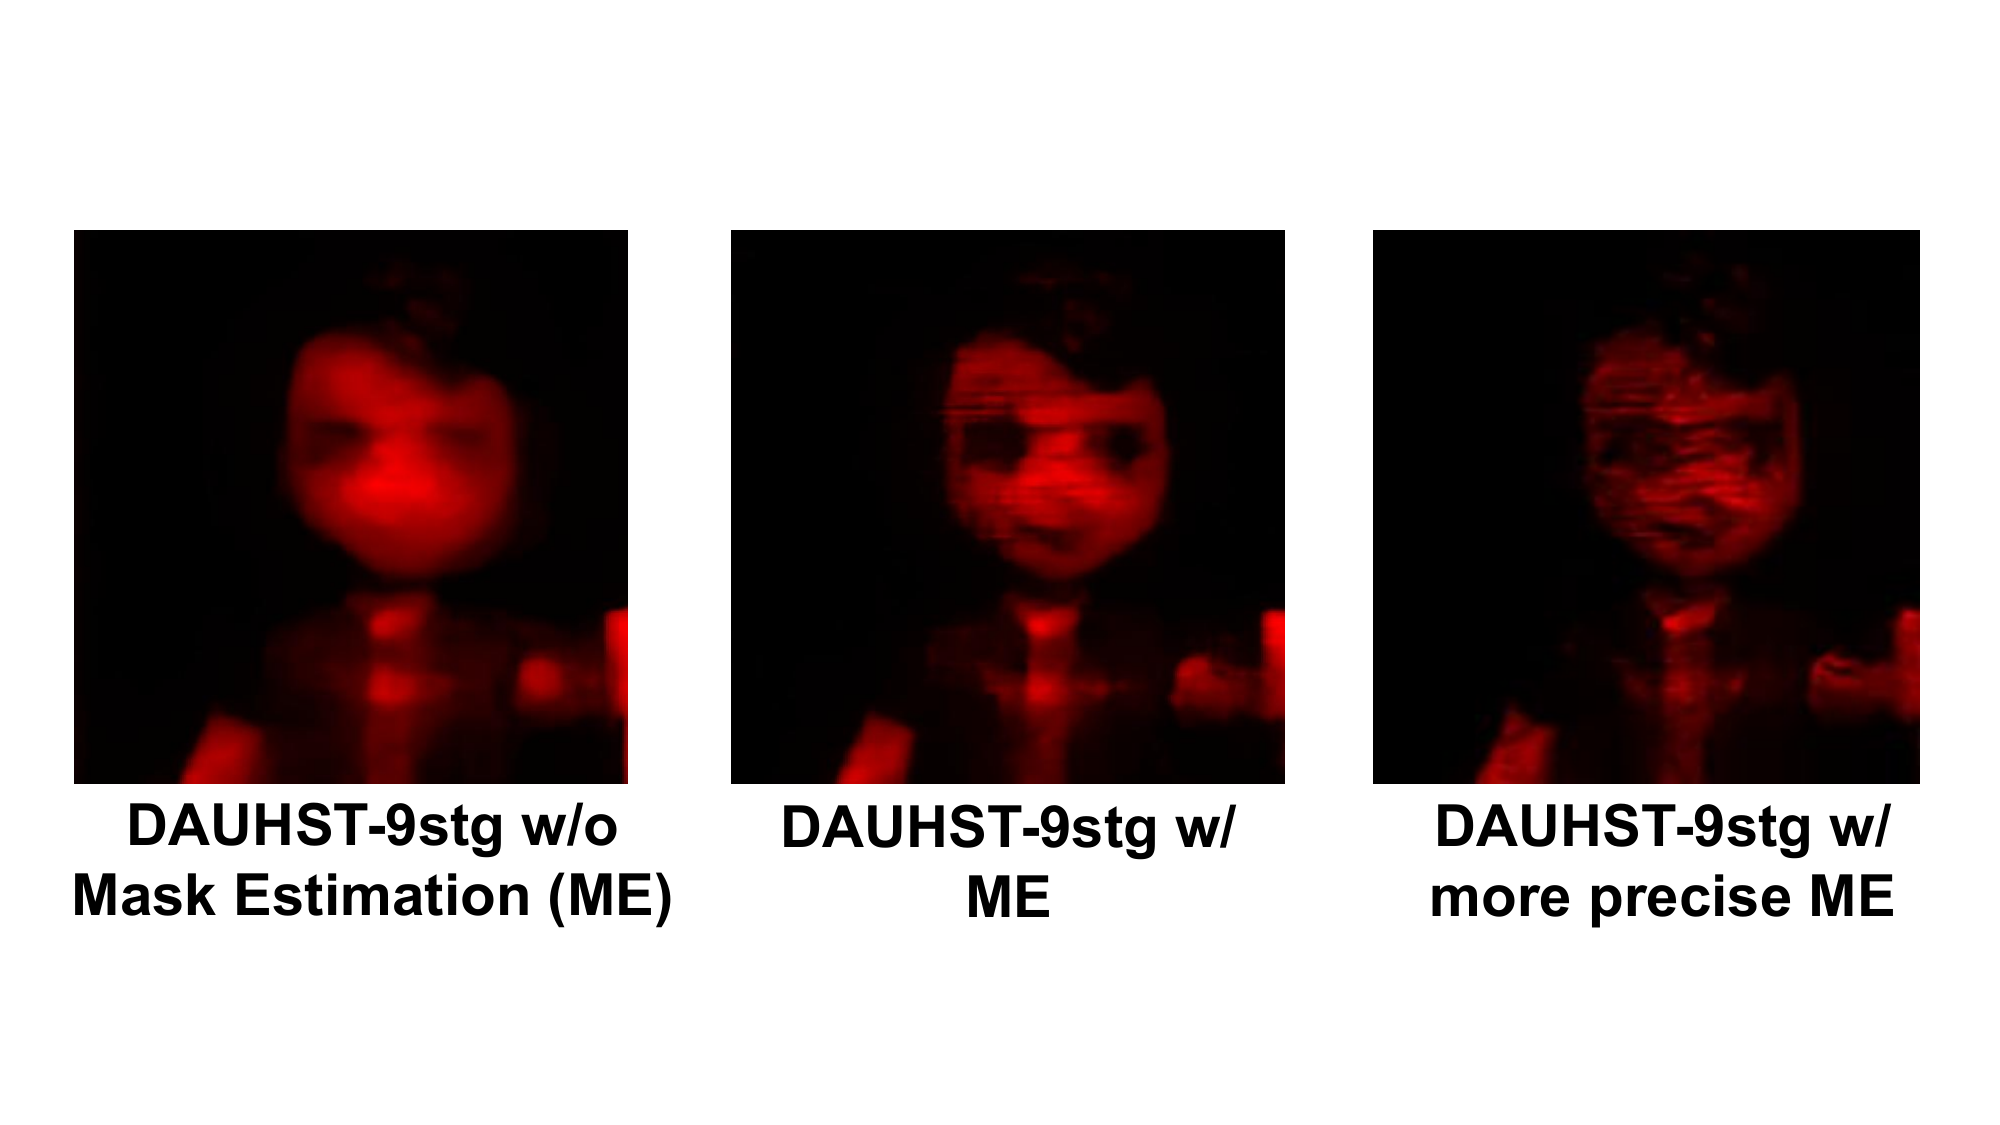}

   \vspace{-2mm}
   \caption{Visual comparisons of DAUHST with, without, and with more precise mask estimation (ME) module, showing the influence of the mask degradation estimation in DAUHST}
    \vspace{-5mm}
   \label{fig:dauhst2}
\end{figure}

As shown in \ref{fig:dauhst2}, we observe that when the mask degradation estimation module is not utilized, the resulting images appear smoother but lose significant detail. In contrast, using the original parameter estimation module better reconstructs details such as the mouth and eyes, but at the cost of introducing some unexpected noise. Besides, when employing the more precise parameter estimation method in \cite{dernn}, the noise becomes so pronounced that the entire facial reconstruction collapses completely.

This result validates our previous conclusion: the reconstruction process of real-world scenes means a balance between real noise loss and compression loss. While in the simulation scenario, leveraging the mask degradation pattern for parameter estimation can effectively reduce compression loss and improve reconstruction outcomes, it inadvertently diminishes the model's ability to handle real noise. When this balance is excessively skewed toward either side, significant issues (detail loss or noise) would arise in the reconstruction of real-world scenes.

\section{Masked Training Strategy}
\subsection{The ratio of 0-1 Mask}

In our masked training method, the proportion of zeros in the mask serves as a critical parameter for balancing compression loss and noise loss. We conducted experiments with three different proportions to compare their results, as detailed below.

\begin{figure}[t]
  \centering
  \hspace{-2.5mm}
   \includegraphics[width=0.98\linewidth]{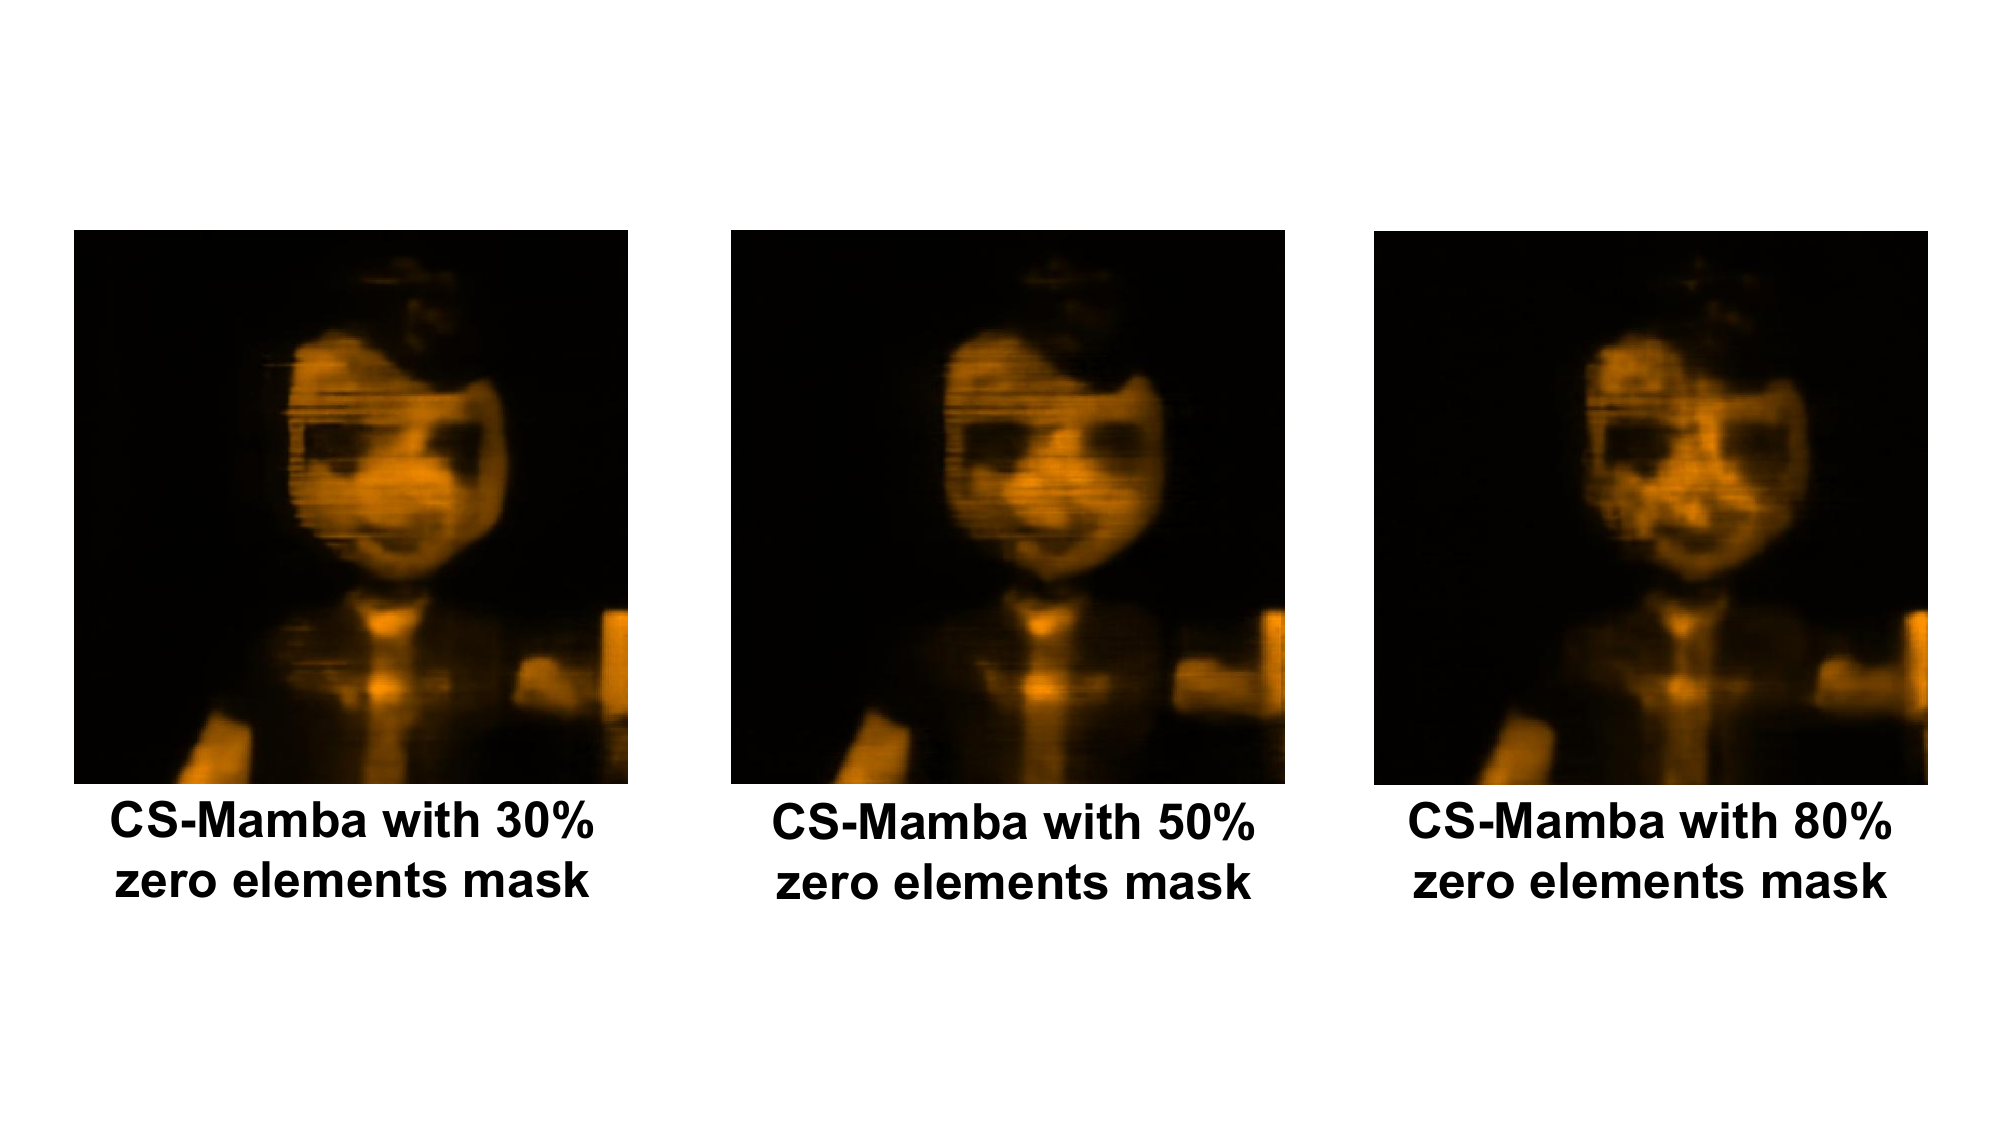}

   \vspace{-2mm}
   \caption{Visual comparisons of CS-Mamba using mask in different 0 ratios}
    \vspace{-5mm}
   \label{fig:01ratio}
\end{figure}

From Figure \ref{fig:01ratio}, we can observe that while the results with a 30\% zero-ratio retain most of the information, they still exhibit noticeable horizontal striped noise. In contrast, the results with an 80\% zero-ratio suffer from a significant loss of original image information, leading to a decline in visual quality. So we finally adopted CS-Mamba with a 50\% zero-ratio mask as our method.

\subsection{The generalizability of masked training}

Our masked training method is not limited to improving the performance of the proposed CS-Mamba model. In fact, this approach enhances the generalization ability of all models, particularly those that leverage coded aperture degradation priors. It proves highly effective in strengthening the robustness of such models against real-world noise like \cite{dernn}, \cite{rdluf}, \cite{padut}, \cite{dernn}, \cite{mst}, \cite{cst}, \cite{herosnet}, \cite{hdnet}.

\begin{figure}[hbp]
  \centering
  \hspace{-2.5mm}
   \includegraphics[width=0.98\linewidth]{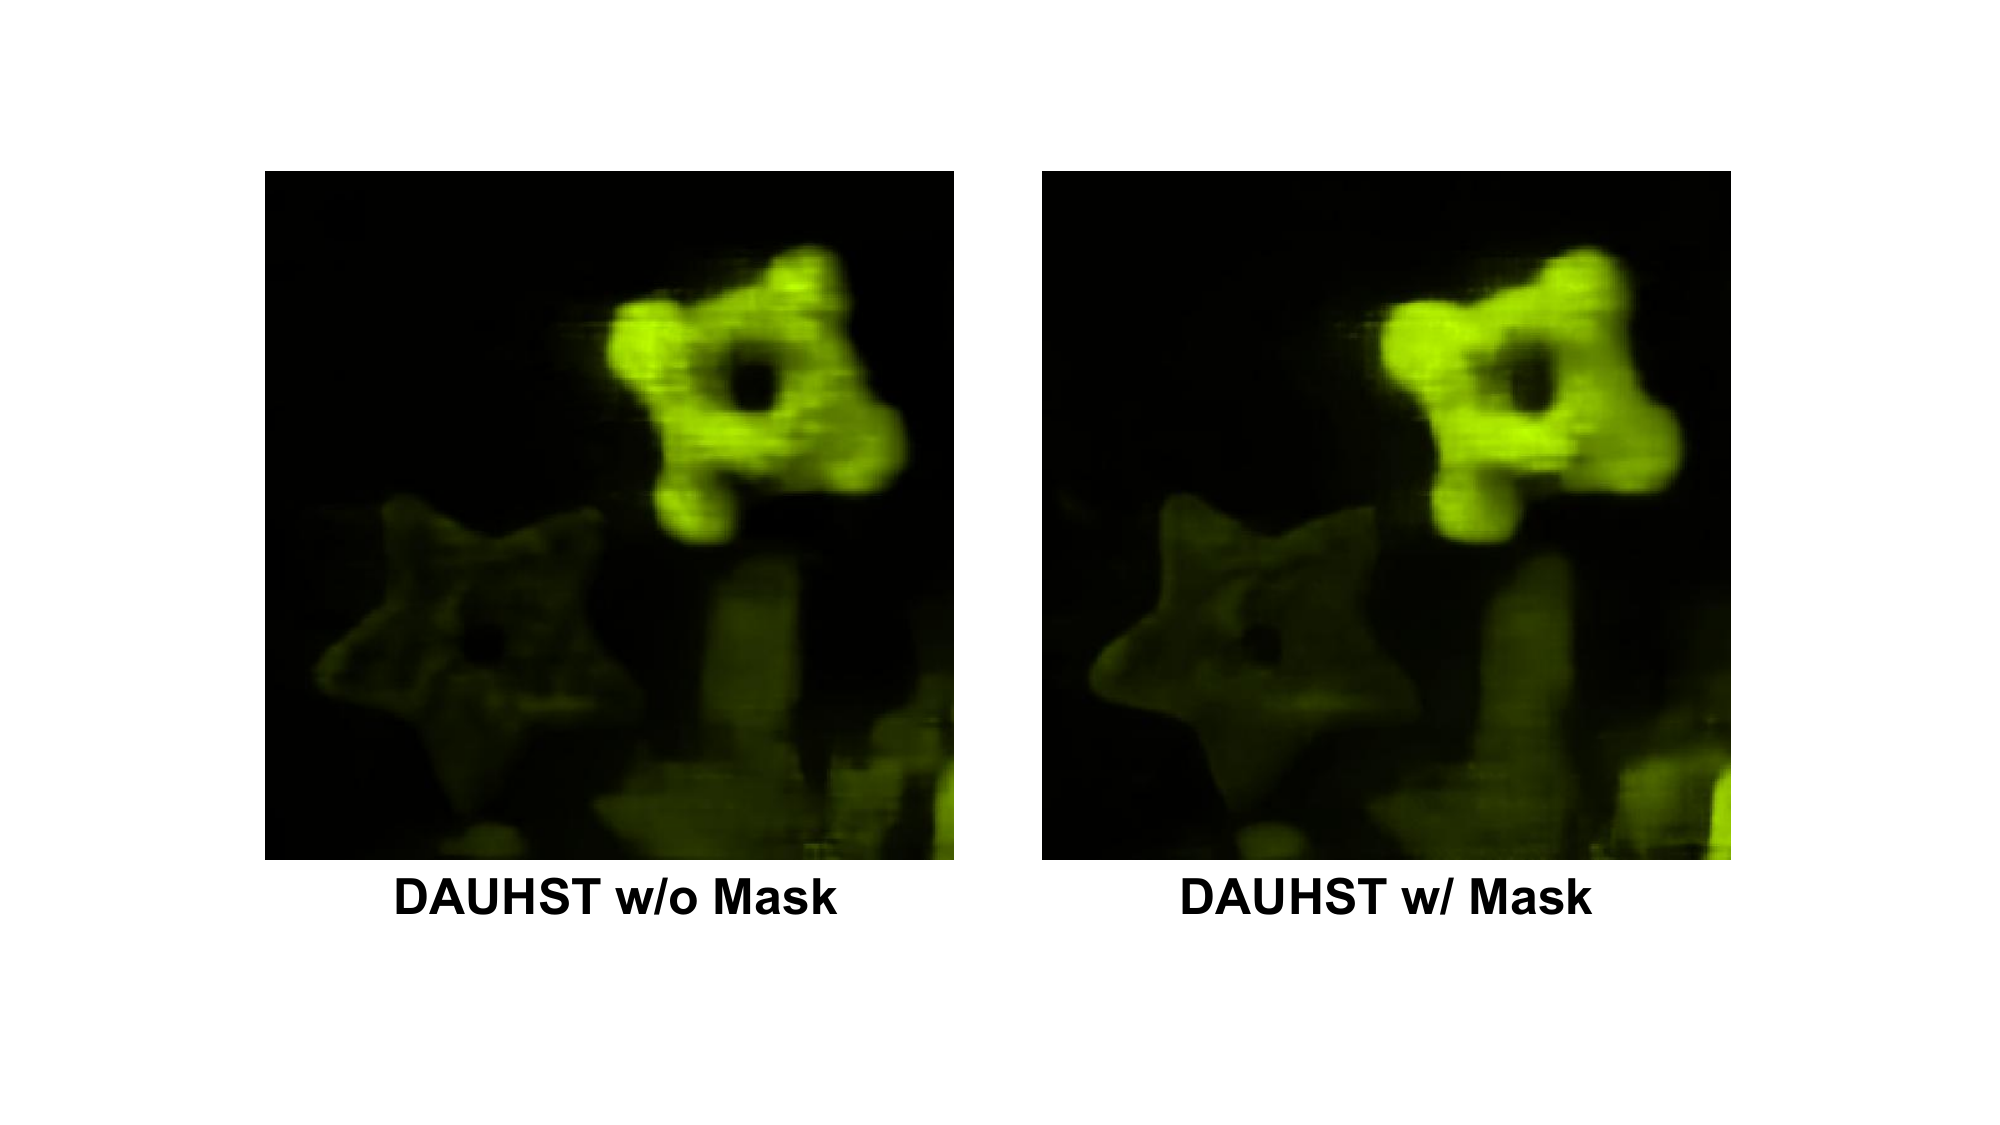}

   \vspace{-2mm}
   \caption{Visual comparisons of DAUHST w/ and w/o mask on scene 1}
    \vspace{-5mm}
   \label{fig:dauhstwithmask}
\end{figure}

\begin{figure*}[hbp]
        \vspace{-3mm}
	% \captionsetup{font=small}
	\centering
	% \scriptsize
        % \Large
	\renewcommand{\h}{0.105}

	\renewcommand{\g}{-0.7mm}
	\renewcommand{\tabcolsep}{1.8pt}
	
        \resizebox{1\linewidth}{!} {
		\begin{tabular}{cc}			
			\renewcommand{\name}{figs/real/}
			\renewcommand{\h}{0.5}
			\renewcommand{\w}{0.5}
			\begin{tabular}{cc}
                    \Huge
				\begin{adjustbox}{valign=t}
					\begin{tabular}{cc}%
		         	\includegraphics[trim={0 0 0 0 },clip, width=0.75\textwidth]{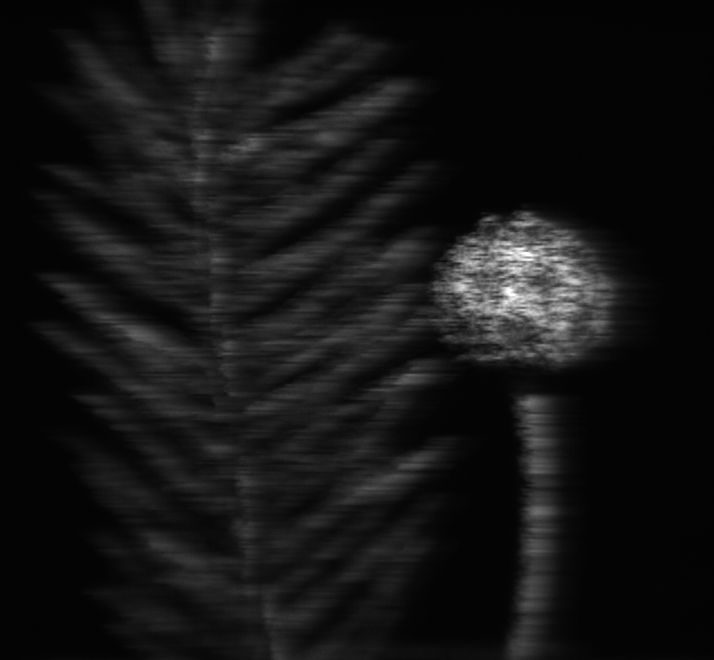}
						\\
						\resizebox{0.55\textwidth}{!}{Real Measurement}
                            \\
                            \includegraphics[trim={0 0 0 0 },clip, width=0.75\textwidth]{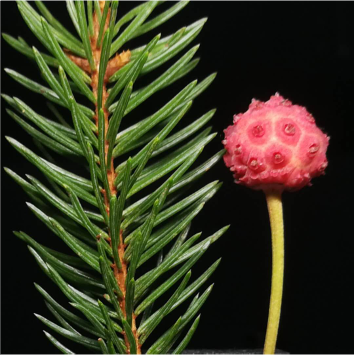}
                            \\
						\resizebox{0.55\textwidth}{!}{Ground Truth}
					\end{tabular}
				\end{adjustbox}
				\begin{adjustbox}{valign=t}
					\begin{tabular}{cccccc}
                        \includegraphics[clip,height=\h \textwidth, width=\w \textwidth]{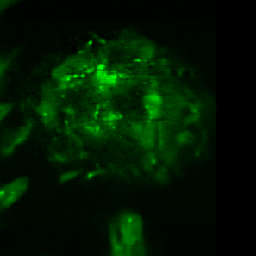} \hspace{\g} & 	
						\includegraphics[clip,height=\h \textwidth, width=\w \textwidth]{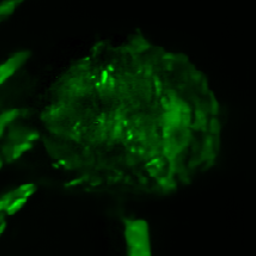} \hspace{\g} &	
						\includegraphics[clip,height=\h \textwidth, width=\w \textwidth]{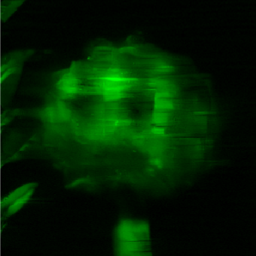} \hspace{\g} &
      					\includegraphics[clip,height=\h \textwidth, width=\w \textwidth]{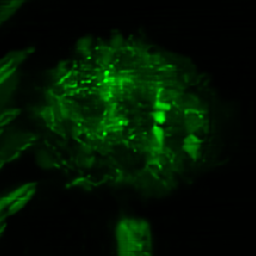} \hspace{\g} &	
						\includegraphics[clip,height=\h \textwidth, width=\w \textwidth]{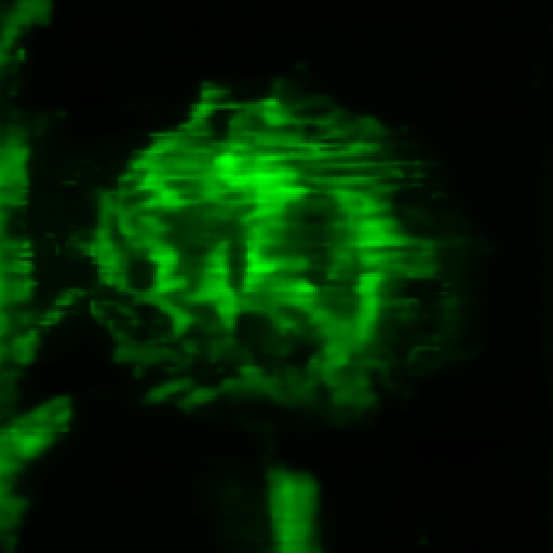} \hspace{\g} &		
						\includegraphics[clip,height=\h \textwidth, width=\w \textwidth]{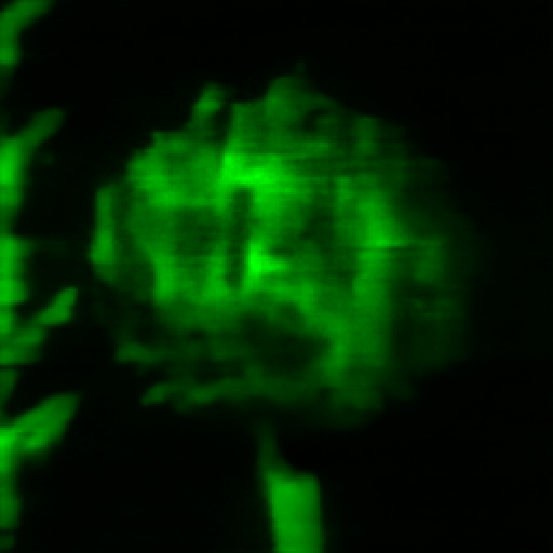}
                        \hspace{\g}

                        \\
      					\includegraphics[clip,height=\h \textwidth, width=\w \textwidth]{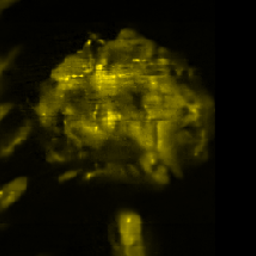} \hspace{\g} & 	
						\includegraphics[clip,height=\h \textwidth, width=\w \textwidth]{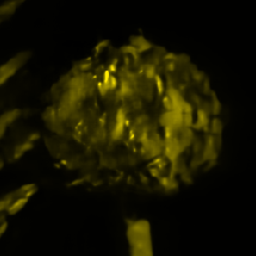} \hspace{\g} &	
						\includegraphics[clip,height=\h \textwidth, width=\w \textwidth]{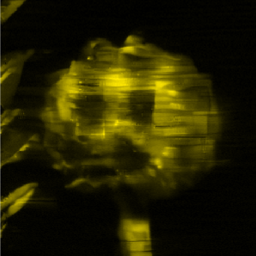} \hspace{\g} &
      					\includegraphics[clip,height=\h \textwidth, width=\w \textwidth]{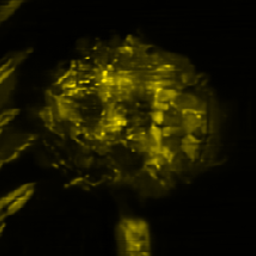} \hspace{\g} &		 
						\includegraphics[clip,height=\h \textwidth, width=\w \textwidth]{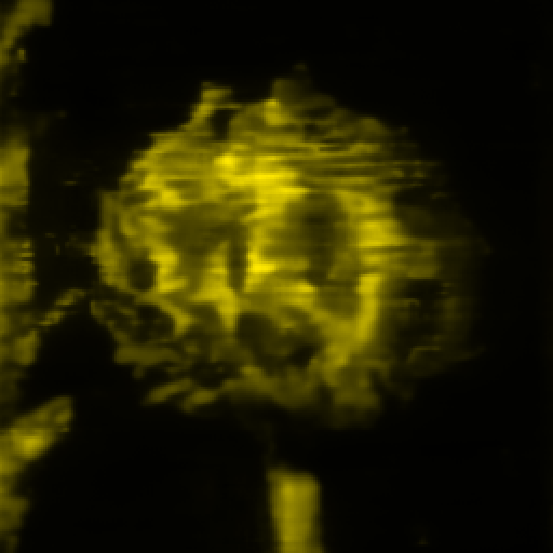} \hspace{\g} &		
						\includegraphics[clip,height=\h \textwidth, width=\w \textwidth]{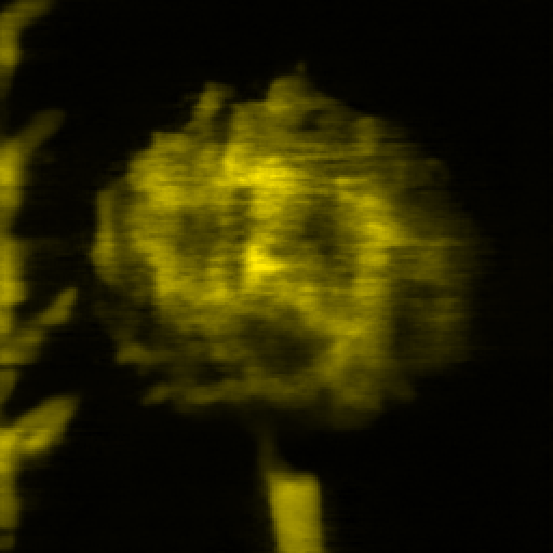}
                        \hspace{\g}

                         \\
      					\includegraphics[clip,height=\h \textwidth, width=\w \textwidth]{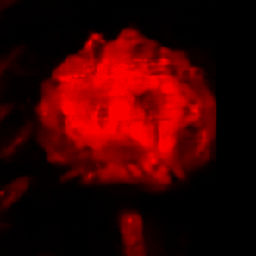} \hspace{\g} & 	
						\includegraphics[clip,height=\h \textwidth, width=\w \textwidth]{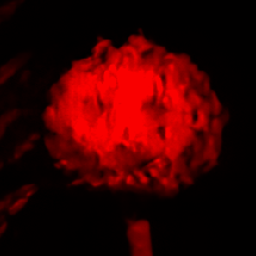} \hspace{\g} &	
						\includegraphics[clip,height=\h \textwidth, width=\w \textwidth]{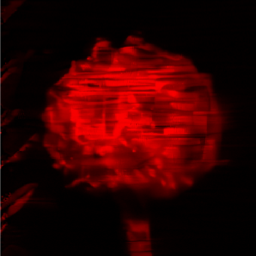} \hspace{\g} &
      					\includegraphics[clip,height=\h \textwidth, width=\w \textwidth]{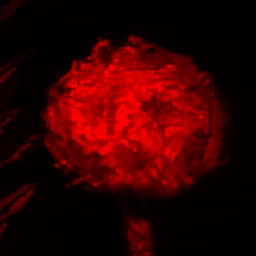} \hspace{\g} &	  
						\includegraphics[clip,height=\h \textwidth, width=\w \textwidth]{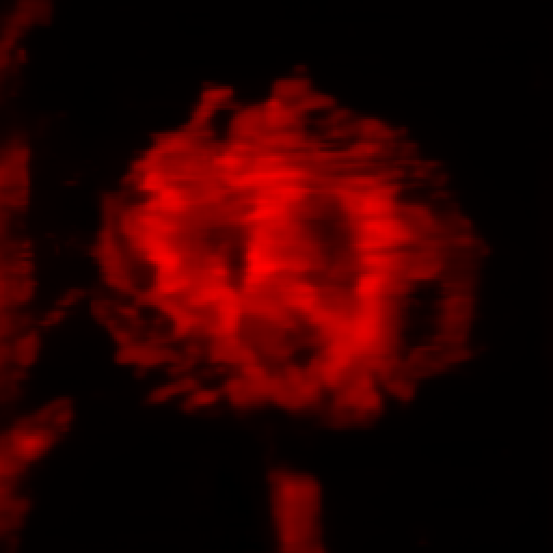} \hspace{\g} &		
						\includegraphics[clip,height=\h \textwidth, width=\w \textwidth]{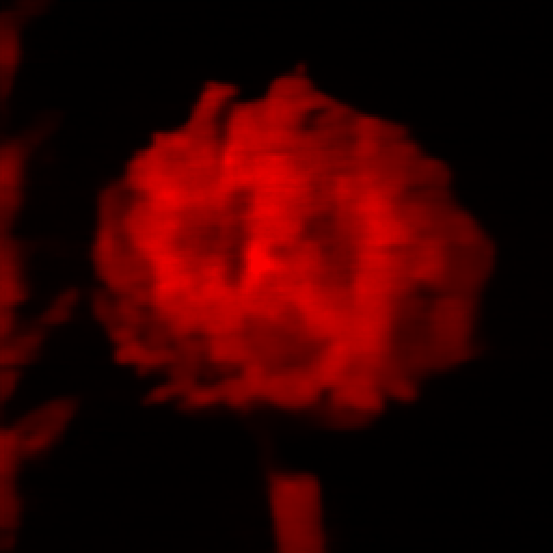}
                        \hspace{\g} \\
                        \resizebox{0.27\textwidth}{!}{GAP-Net} & \resizebox{0.27\textwidth}{!}{DGSMP } & \resizebox{0.27\textwidth}{!}{DiffSCI } & \resizebox{0.27\textwidth}{!}{DAUHST} & \resizebox{0.37\textwidth}{!}{\textbf{Ours (3stg)}} & \resizebox{0.42\textwidth}{!}{\textbf{Ours (Mask)} }
                        
					\end{tabular}
				\end{adjustbox}
			\end{tabular}	
		\end{tabular}
  
	}
	% \vspace{-4mm}
        \vspace{-4mm}
	\caption{Visual comparison of SCI reconstruction methods on real $Scene$ 2.} %
	\label{fig_real_s2}
    \vspace{-6mm}
\end{figure*}

As shown in Figure 3, the reconstruction result obtained using our masked training strategy in \cite{dauhst} is significantly superior to the one without this method, effectively mitigating the noise issues. 
This demonstrates that our method is not only effective in our CS-Mamba model but also useful in other models that leverage the information in the coded aperture.

\section{Other Visual Results of CS-Mamba}

In addition to the comparisons previously provided in our paper, we also present results for another real scenario and another simulation scenario. Due to the more irregular features of the additional real scene, the improvements may appear less discernible. However, upon closer inspection, the enhancements achieved through the use of masked training can still be observed. The results are illustrated in Figure \ref{fig_real_s2}, \ref{fig_kaist_s1}.

\begin{figure*}[!t]
	\centering
	\renewcommand{\h}{0.105}

	\renewcommand{\g}{-0.7mm}
	\renewcommand{\tabcolsep}{1.8pt}

        \resizebox{1\linewidth}{!} {
		\begin{tabular}{cc}			
			\renewcommand{\name}{figs/simulation/}
			\renewcommand{\h}{0.5}
			\renewcommand{\w}{0.5}
			\begin{tabular}{cc}
                    \Huge
				\begin{adjustbox}{valign=t}
					\begin{tabular}{cc}%
		         	\includegraphics[trim={0 0 0 0 },clip, width=1.09\textwidth]{\name measurement/meas1.png}
						\\
						\resizebox{0.3\textwidth}{!}{Scene 2}
					\end{tabular}
				\end{adjustbox}
				\begin{adjustbox}{valign=t}
					\begin{tabular}{ccccccc} 

                        \includegraphics[trim={80 130 120 70  },clip,height=\h \textwidth, width=\w \textwidth]{\name measurement/meas1.png} \hspace{\g} &
                        \includegraphics[trim={80 130 120 70  }, clip,height=\h \textwidth, width=\w \textwidth]{\name gt/frame1channel8.png} \hspace{\g} &
                        \includegraphics[trim={80 130 120 70  }, clip,height=\h \textwidth, width=\w \textwidth]{\name admm_net/frame1channel8.png} \hspace{\g} &
						\includegraphics[trim={80 130 120 70  }, clip,height=\h \textwidth, width=\w \textwidth]{\name cst_l_plus/frame1channel8.png} \hspace{\g} &
      					\includegraphics[trim={80 130 120 70  }, clip,height=\h \textwidth, width=\w \textwidth]{\name dgsmp/frame1channel8.png} \hspace{\g} &
						\includegraphics[trim={80 130 120 70  }, clip,height=\h \textwidth, width=\w \textwidth]{\name dip_hsi/frame1channel8.png} \hspace{\g} &
 						\includegraphics[trim={80 130 120 70  }, clip,height=\h \textwidth, width=\w \textwidth]{\name hdnet/frame1channel8.png} \hspace{\g} 
					  \\
                        \resizebox{0.22\textwidth}{!}{Meas } &\resizebox{0.32\textwidth}{!}{GT Patch } & \resizebox{0.4\textwidth}{!}{ADMM-Net } & \resizebox{0.25\textwidth}{!}{CST-L+} & \resizebox{0.3\textwidth}{!}{DGSMP } & \resizebox{0.3\textwidth}{!}{DIP-HSI}  & \resizebox{0.25\textwidth}{!}{HDNet } 
                            \\
      						
					   \includegraphics[trim= {80 130 120 70  }, clip,height=\h \textwidth, width=\w \textwidth]{\name gap_net/frame1channel8.png} \hspace{\g} &	\includegraphics[trim={80 130 120 70  }, clip,height=\h \textwidth, width=\w \textwidth]{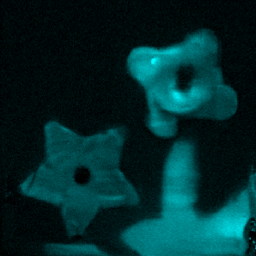} \hspace{\g} &
						\includegraphics[trim={80 130 120 70  }, clip,height=\h \textwidth, width=\w \textwidth]{\name lambda_net/frame1channel8.png} \hspace{\g} &
      					\includegraphics[trim={80 130 120 70  }, clip,height=\h \textwidth, width=\w \textwidth]{\name mst_l/frame1channel8.png} \hspace{\g} &

                        \includegraphics[trim={80 130 120 70  }, clip,height=\h \textwidth, width=\w \textwidth]{\name dauhst/frame1channel8.png} \hspace{\g} &	
						\includegraphics[trim={80 130 120 70  }, clip,height=\h \textwidth, width=\w \textwidth]{\name padut/frame1channel8.png} \hspace{\g} &		
						\includegraphics[trim={80 130 120 70  }, clip,height=\h \textwidth, width=\w \textwidth]{\name cs-mamba/frame1channel8.png} \hspace{\g} \\
                        \resizebox{0.33\textwidth}{!}{GAP-Net }&
                        \resizebox{0.3\textwidth}{!}{DiffSCI } & \resizebox{0.25\textwidth}{!}{$\lambda$-Net } & \resizebox{0.25\textwidth}{!}{MST-L} & \resizebox{0.3\textwidth}{!}{DAUHST} & \resizebox{0.3\textwidth}{!}{PADUT } &
                        \resizebox{0.45\textwidth}{!}{\textbf{CS-Mamba} }
					\end{tabular}
				\end{adjustbox}
			\end{tabular}	
		\end{tabular}
}
	\vspace{-3mm}
	\caption{Visual comparison on $\operatorname{KAIST}$ at wavelength 487.0nm.}
    \vspace{-5mm}
	\label{fig_kaist_s1}
\end{figure*}

% \label{sec:rationale}
% % 
% Having the supplementary compiled together with the main paper means that:
% % 
% \begin{itemize}
% \item The supplementary can back-reference sections of the main paper, for example, we can refer to \cref{sec:intro};
% \item The main paper can forward reference sub-sections within the supplementary explicitly (e.g. referring to a particular experiment); 
% \item When submitted to arXiv, the supplementary will already included at the end of the paper.
% \end{itemize}
% % 
% To split the supplementary pages from the main paper, you can use \href{https://support.apple.com/en-ca/guide/preview/prvw11793/mac#:~:text=Delete%20a%20page%20from%20a,or%20choose%20Edit%20%3E%20Delete).}{Preview (on macOS)}, \href{https://www.adobe.com/acrobat/how-to/delete-pages-from-pdf.html#:~:text=Choose%20%E2%80%9CTools%E2%80%9D%20%3E%20%E2%80%9COrganize,or%20pages%20from%20the%20file.}{Adobe Acrobat} (on all OSs), as well as \href{https://superuser.com/questions/517986/is-it-possible-to-delete-some-pages-of-a-pdf-document}{command line tools}.
